# Supplementary material for: Stochastic resonance on the transverse displacement of swimmers in an oscillatory shear flow
Source: arXiv:1208.5214 source file (2012-09-05)
Supplement: Supplementary file 1 [file SR_Supporting_information.pdf]

# Supporting material for: Stochastic resonance on the transverse displacement of swimmers in an oscillatory shear flow

Francisca Guzmán-Lastra and Rodrigo Soto

*Departamento de Física, FCFM, Universidad de Chile, Santiago, Chile*

(Dated: August 26, 2012)

## A. The orientation

The numerical solution of the swimmer equations of motion, shows that due to the polar symmetry, the odd averages of the swimmer director, velocity and displacements vanish when averaged over the noise and one period. To quantify the degree of orientation, averages of quadratic quantities are considered. The quadratic averages of the director vector $\hat{n}$, $\langle n_x^2\rangle$, $\langle n_y^2\rangle$ and $\langle n_z^2\rangle$, computed for long times, after the transients effects of the initial condition are lost, are shown in Fig. 1. The swimmer preferentially orients along the $x$ axis for small noise intensities, while it orients isotropically for large noise intensities ($\Gamma/\dot{\gamma}^{\infty} \sim 1$) and $\langle n_x^2\rangle = \langle n_y^2\rangle = \langle n_y^2\rangle = 1/3$.

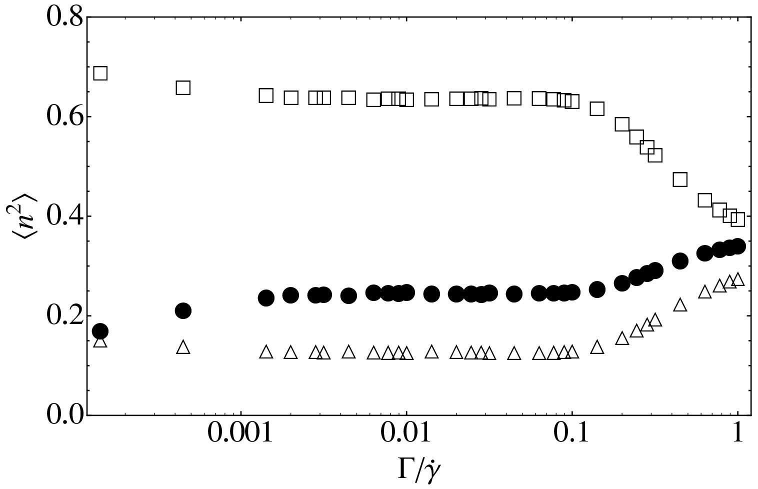


FIG. 1. Quadratic averages of the components of the director vector $\langle n_x^2\rangle$ (squares), $\langle n_y^2\rangle$ (triangles) and $\langle n_z^2\rangle$ (solid circles) as a function of the noise intensity $\Gamma$. The oscillation frequency is $\omega_2$. Similar results are obtained for the other oscillation frequencies.

## B. Resonance for a swimmer with shape parameter $\beta = 0.6$

In the letter, the case of a swimmer with a shape parameter $\beta = 1$ is discussed in detail. It is interesting to study the case of other elongated swimmers (i.e., $\beta > 0$) that are not infinitely thin. Here, we present the case of an elongated swimmer with $\beta = 0.6$. Figure 2 shows the average squared coarse grained displacements as a function of the noise intensities in the $z$ direction and in the $y$ direction. The stochastic resonance is present also. The

resonant noise intensity is smaller and it is approximately $\Gamma/\dot{\gamma}^\infty \sim 0.001$ for $\omega_3/\dot{\gamma}^\infty = \pi/5$. The transverse resonant displacement is smaller than in the case $\beta = 1$ at the same frequency.

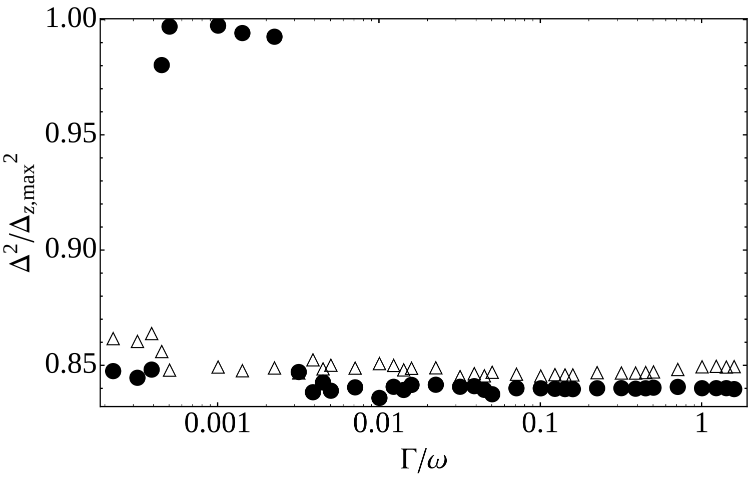


FIG. 2. Average squared coarse grained displacements as a function of the noise intensity $\Gamma$ for a swimmer characterized by a shape parameter $\beta = 0.6$. The linear vertical scale has been rescaled for each frequency to the maximum value of $\langle \Delta_z^2 \rangle$. The oscillation frequency is $\omega_3$. $\langle \Delta_z^2 \rangle$ (solid circles) and $\langle \Delta_y^2 \rangle$ (open triangles).
